# Supplementary material for: Instabilities in Multi-Asset and Multi-Agent Market Impact Games
Source: arXiv:2004.03546 source file (2021-11-27)
Supplement: Supplementary file 1 [file appendix_shape_4agent.tex]

\section{The role of initial inventories in multi-agent market impact games}\label{app_shape_analysis}

% What happens if the agents have not 
% {\color{blue} identical inventories}?

Here we analyse how the equilibrium solution is affected by the inventories of the agents. 
We consider $J=4$ Fundamentalist sellers having different initial inventory. In all cases we fix the total initial inventory to $X_0^1+X_0^2+X_0^3+X_0^4=4$. As a benchmark case we consider the case of equal inventories $X_0^i=1$ (see top left panel of Figure \ref{fig_agents_V1_J4}). When the inventory of one seller is  $1/2$ and equal to $7/6$ for the three remaining ones, we observe that the solution of the small seller tends to concentrate more orders at the beginning of the session (top right panel of Fig. \ref{fig_agents_V1_J4}). By reducing the inventory of the small seller, setting her inventory equal to $1/10$ in competition with other three sellers with inventory  equal to $13/10$, the behavior of the former becomes more similar to that of an Arbitrageur (see bottom left panel of Fig. \ref{fig_agents_V1_J4}). In fact, the optimal solution is to place all positive orders at the beginning and wait the end of the trading session to liquidate the excess volume, exploiting the position of the big Fundamentalists.
Also we observe that in contrast to 
the $J=2$ case the shape of the solution for big sellers is not affected by the presence of the small one. 

\begin{figure}[t]
\centering
{\includegraphics[width=0.48\textwidth]{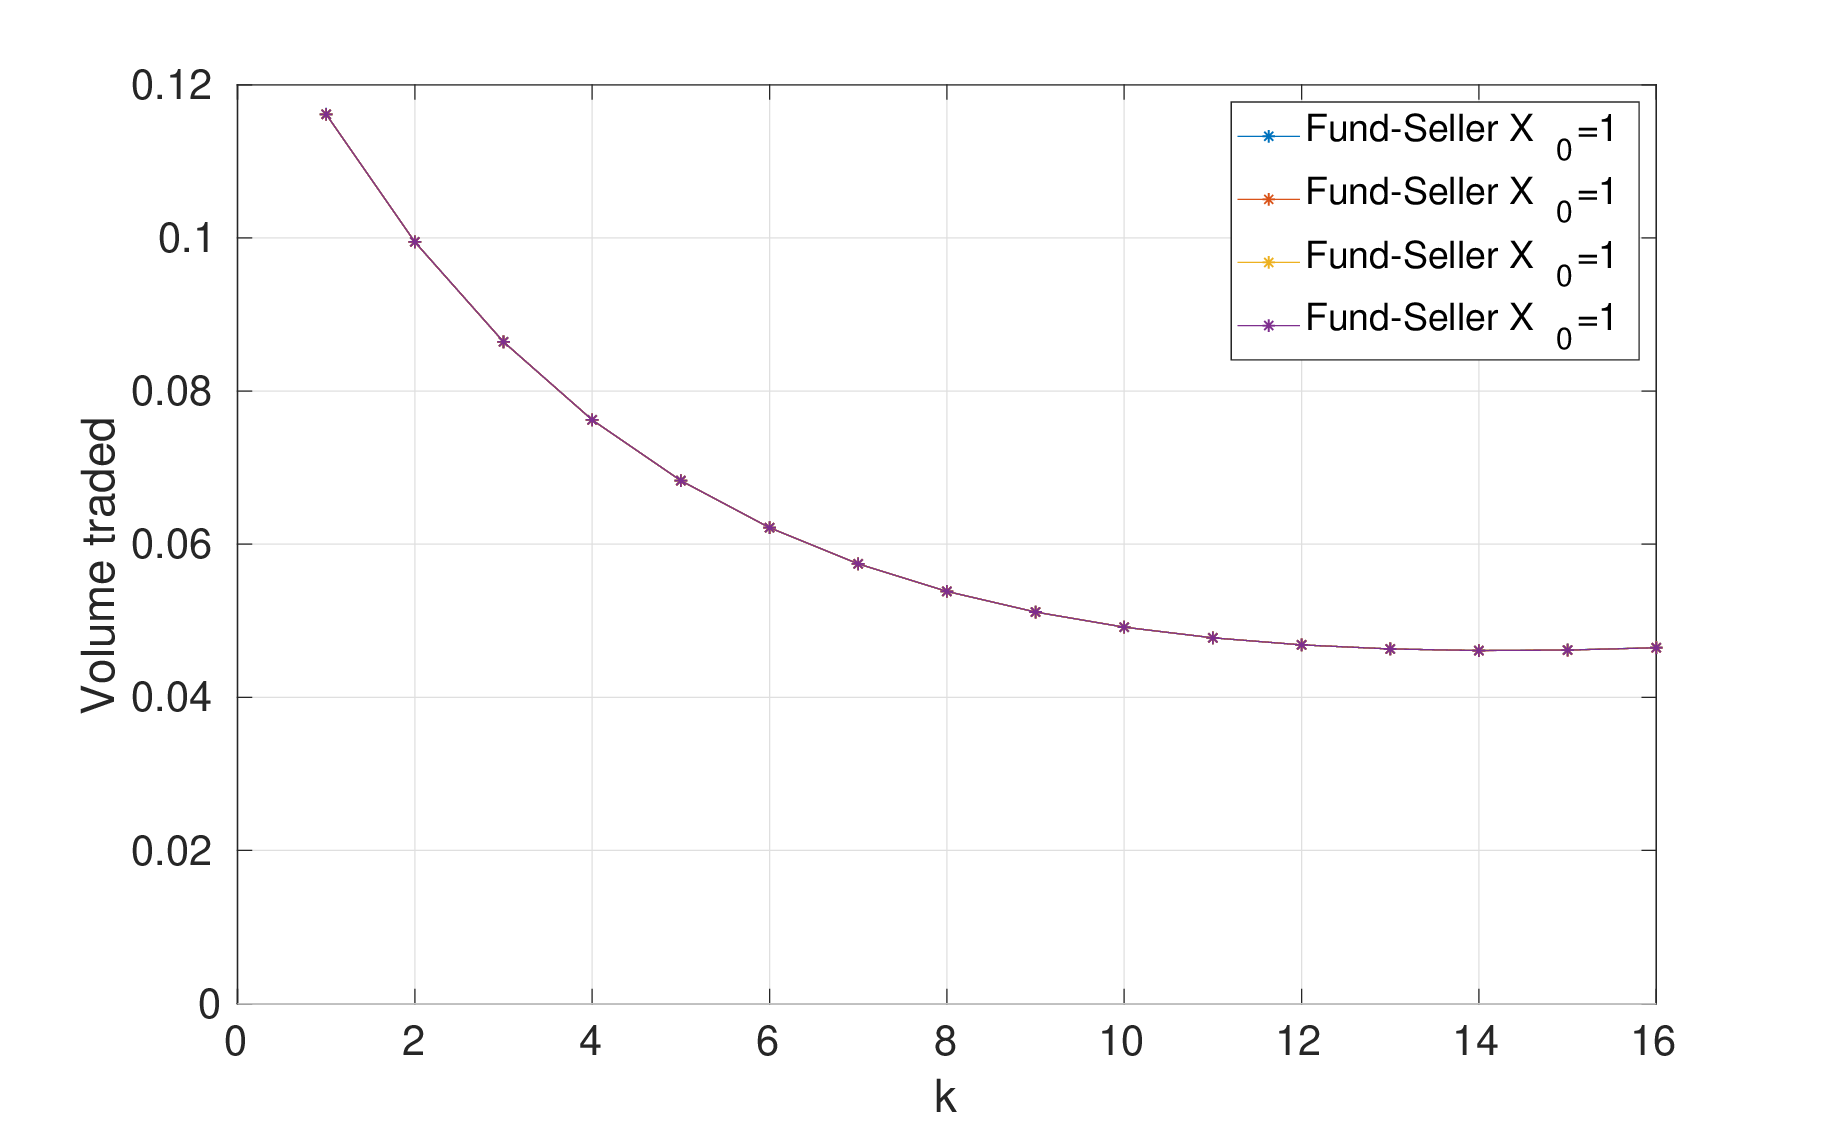}}
{\includegraphics[width=0.48\textwidth]{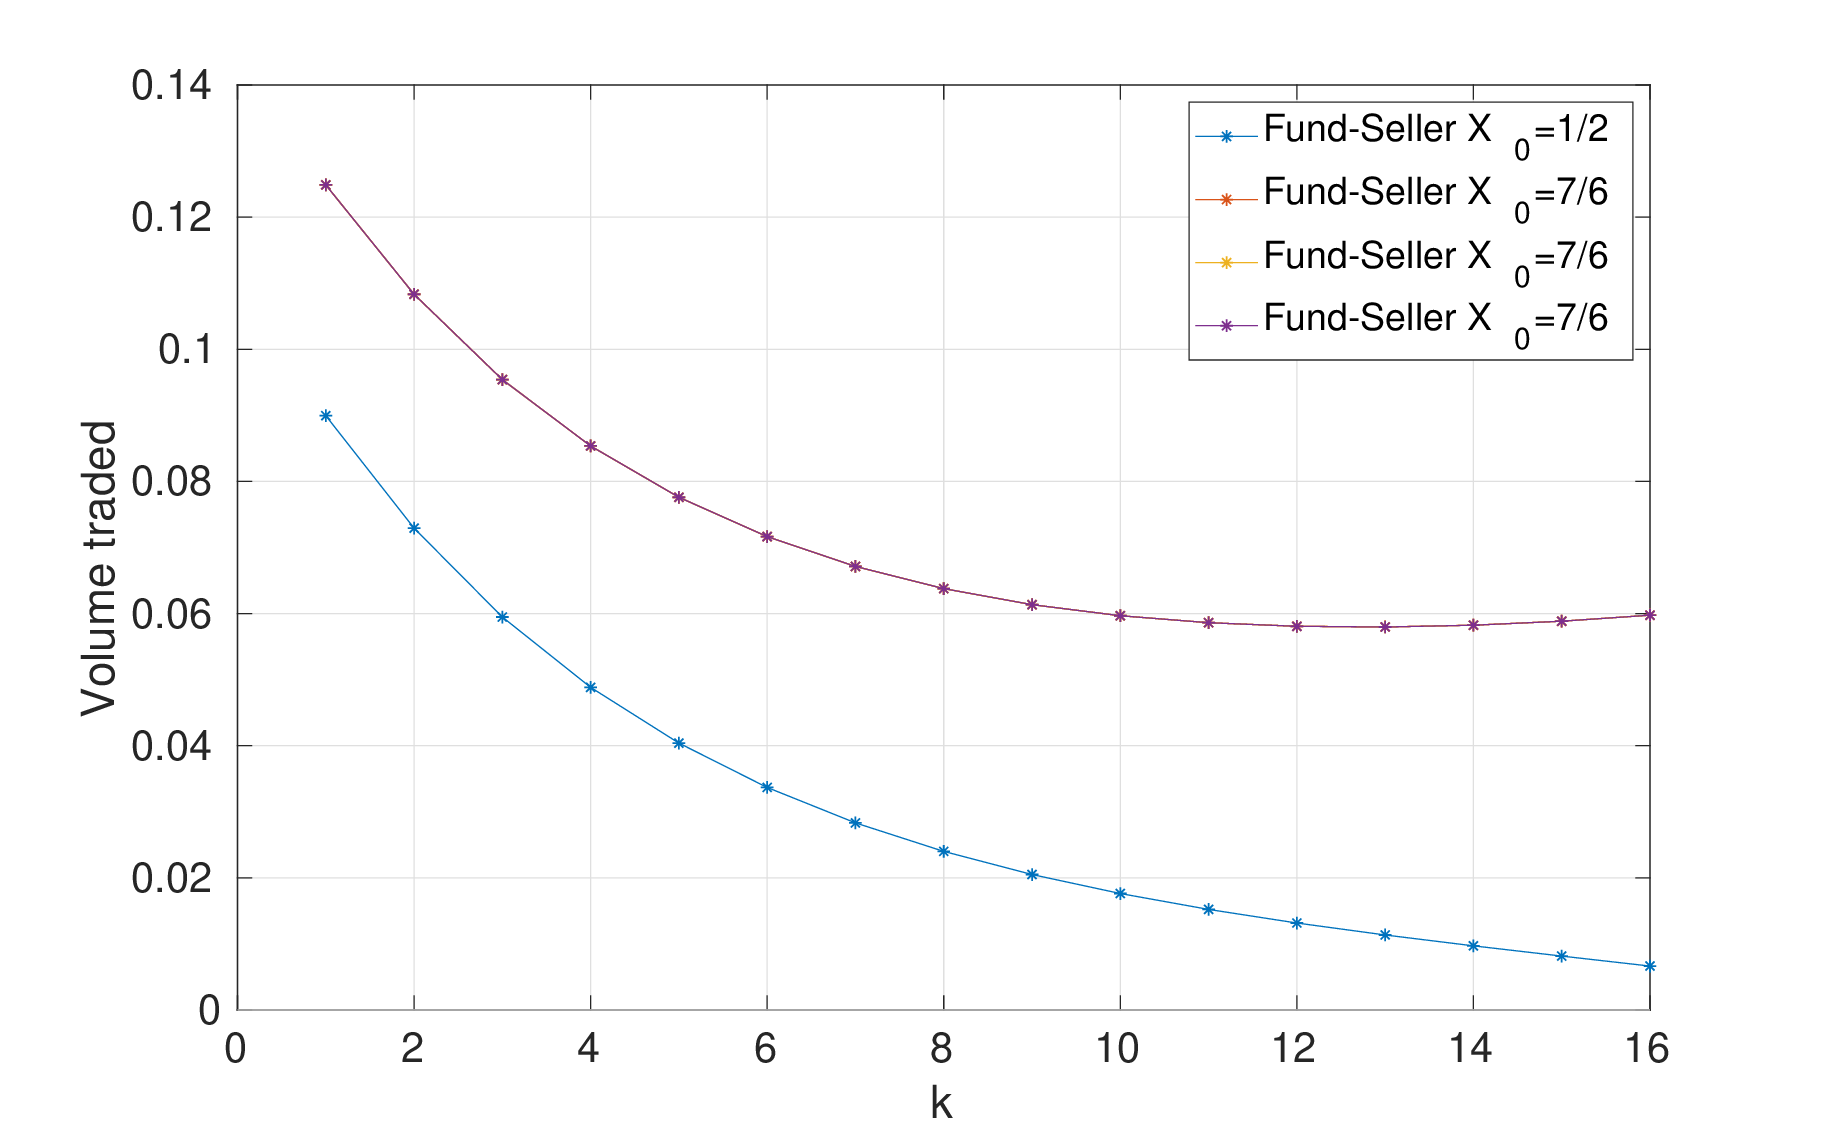}}\\
{\includegraphics[width=0.48\textwidth]{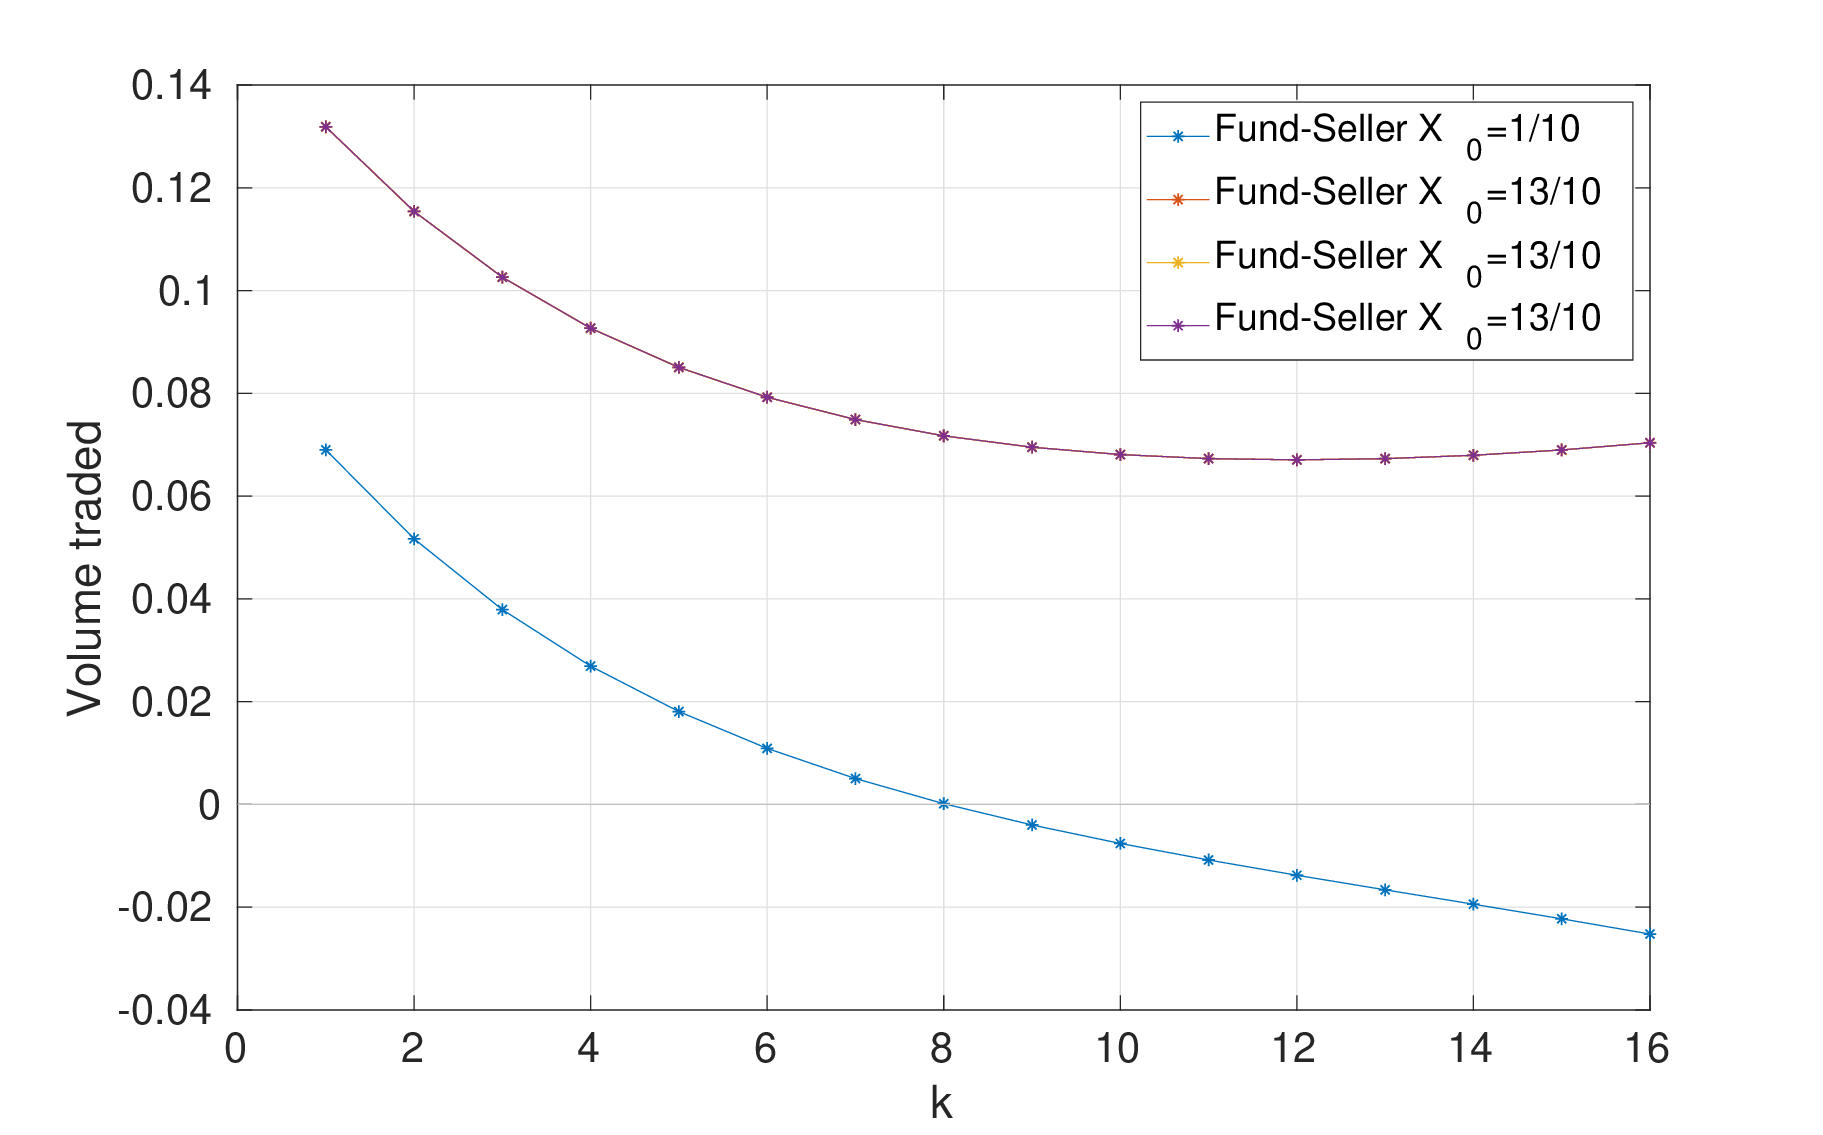}}
{\includegraphics[width=0.48\textwidth]{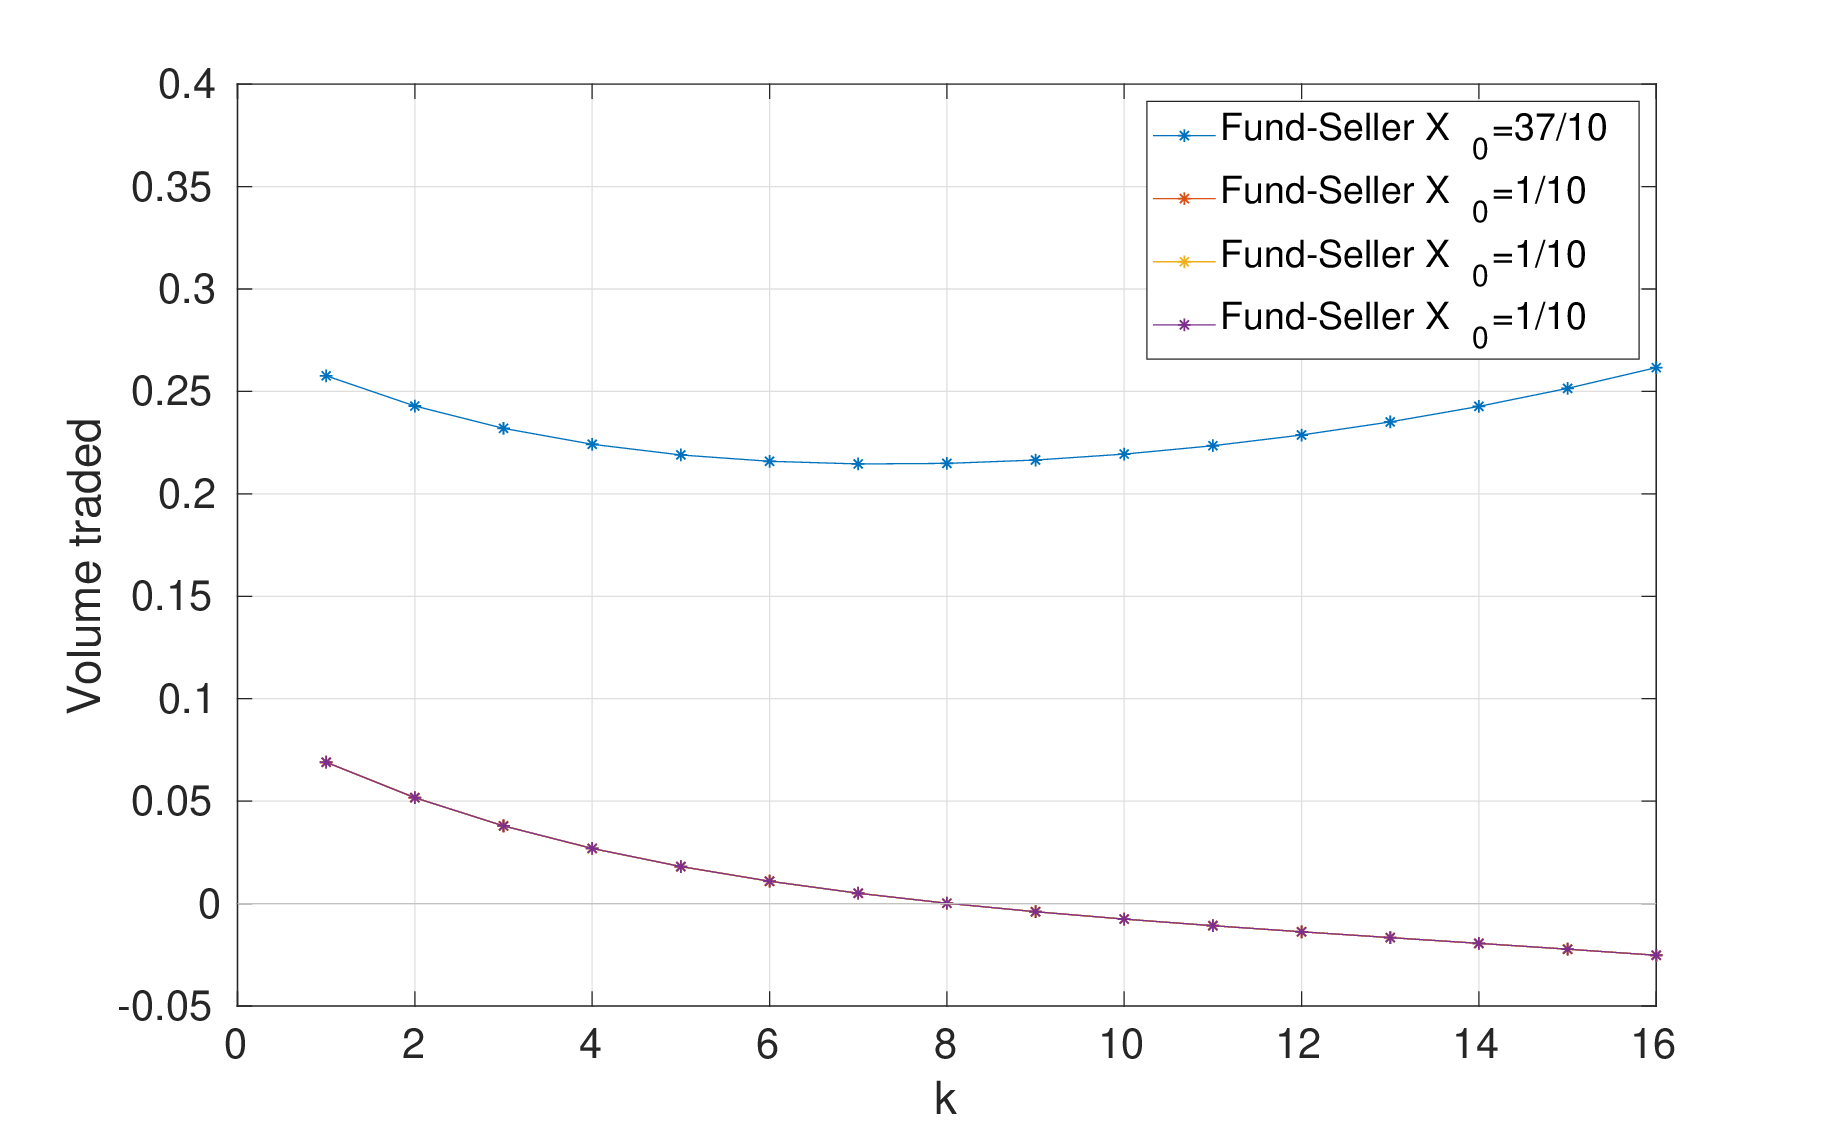}}
\caption{Nash equilibrium for $J=4$ Fundamentalist sellers for four different sets of initial inventory such that the total volume traded is $4$. The time grid has $16$ points, $G(t)=\exp(-t)$, and $\theta=10.$}\label{fig_agents_V1_J4}
\end{figure} 

To get some intuition on this result, we remind that in the two agents case \cite{schied2018market} showed that the solution is characterized by the sum and difference of the inventories, see Equation 
\eqref{eq_1_S&Z} and \eqref{eq_2_S&Z}.
% if the inventories are denoted by $X_0^1$ and 
% $X_0^2$ the equilibrium for agent $1$ and $2$ is given, respectively
% \[
% \begin{split}
% \bm{\xi}_1^*&=\frac{1}{2} (X_0^1 +X_0^2)\bm{v}
% +\frac{1}{2} (X_0^1-X_0^2)\bm{w}
% \\
% \bm{\xi}_2^*&=\frac{1}{2} (X_0^1 +X_0^2)\bm{v}
% -\frac{1}{2} (X_0^1-X_0^2)\bm{w}
% \end{split}
% \]
% where \[
% \begin{split}
%   \bm{v}&=\frac{1}{\bm{e}^T (\Gamma_{\theta}+\widetilde{\Gamma})^{-1}\bm{e}}(\Gamma_{\theta}+\widetilde{\Gamma})^{-1}\bm{e}\\ 
%      \bm{w}&=\frac{1}{\bm{e}^T (\Gamma_{\theta}-\widetilde{\Gamma})^{-1}\bm{e}}(\Gamma_{\theta}-\widetilde{\Gamma})^{-1}\bm{e}.
% \end{split}
% \]
Thus, if the two traders have the same inventory the solution is fully characterized by the vector $\bm{v}$, which is scaled by the sum of the inventories.  Figure 2 of \cite{schied2018market} shows
the shapes of $\bm{v}$ and $\bm{w}$, and we note that  the former is a vector which assigns more trades at the beginning, while $\bm{w}$ tends to concentrate orders at the end of trading session. 
Let us suppose that $X_0^1<X_0^2$, then the solution for trader $1$ is a linear combination of $\bm{v}$ and $\bm{w}$ with opposite signs (thus positive at the beginning and negative at the end), while for the second trader the solution is approximately given by a positive linear combination of
$\bm{v}$ and $\bm{w}$ (an asymmetric U-shape), so that its equilibrium's shape converges to a U-shape. In particular, in the case of $X_0^1<<X_0^2$, at the equilibrium, the first seller will place positive orders at the beginning while at the end he/she will place opposite sign orders.

Let us go back to the $J=4$ case. We have observed how the presence of a single small seller does not
affect the shapes of the big ones.
However, this may be related to market dominance of the big sellers. Indeed, if we analyse the complementary case when there is only one big seller with inventory equal to $37/10$ against three small sellers whose inventories are all equal to $1/10$, we observe
from the bottom right panel of Figure \ref{fig_agents_V1_J4} that the optimal schedule for the big sellers approaches to a U-shape like in the $J=2$ case, while the small agents behaves similarly to Arbitrageurs.

Therefore, in a multi-agent market along with the increasing in competition we have also to take into account another effect which is the market dominance in terms of inventory.
Obviously this effect is masked in the $J=2$ case.
We conclude by conjecturing that when the market is dominated by small agents the optimal schedule for the big sellers approach to a U-shape form, like in the $J=2$ case, while its shape is invariant when market is dominated by sellers with the same inventory volume size.
